# Supplementary material for: A Neural Affinity Framework for Abstract Reasoning: Diagnosing the Compositional Gap in Transformer Architectures via Procedural Task Taxonomy
Source: arXiv:2512.07109 source file (2025-12-08)
Supplement: Supplementary file 1 [file APPENDIX_B_EXTENDED_GLOSSARY.tex]

% Wrapper to include Markdown appendix in LaTeX build
% Requires \usepackage{markdown} in the preamble
\begingroup
\markdownInput{../../APPENDIX/APPENDIX_B_EXTENDED_GLOSSARY.md}
\endgroup
